# Supplementary material for: Direct evidence of void induced structural relaxations in colloidal glass formers
Source: arXiv:2011.02754 ancillary file (2020-11-06)
Supplement: Supplementary file 1 [file supplementary_materials_2020_11_4.pdf]

# Supplementary Material for

## Title: Direct evidence of void induced structural relaxations in colloidal glass formers

Authors: Cho-Tung Yip[1], Masaharu Isobe[2], Chor-Hoi Chan[1], Simiao Ren[1,3], Kin-Ping Wong[3], Qingxiao Huo[1], Chun-Sing Lee[3], Yuen-Hong Tsang[3], Yilong Han[4], Chi-Hang Lam[3]*

**Affiliations:**

[1]School of Science, Harbin Institute of Technology (Shenzhen), Shenzhen 518055, China

[2]Graduate School of Engineering, Nagoya Institute of Technology, Nagoya, 466-8555, Japan.

[3]Department of Applied Physics, Hong Kong Polytechnic University, Hung Hom, Hong Kong, China.

[4]Department of Physics, Hong Kong University of Science and Technology, Clear Water Bay, Hong Kong, China.

*Correspondence to: E-mail: C.H.Lam@polyu.edu.hk

**This PDF file includes:**

Materials and Methods
Supplementary Results on Glassy Colloidal Systems
Supplementary Results on Glass-crystal Coexisting Systems
Figures S1 to S23

## 1. Materials and Methods

### 1.1. Experimental Colloidal Systems

We use polymethyl methacrylate (PMMA) colloidal particles for all of the experiments in this work. Each particle has a thin coating of trihydroxy octadecylsilane, which prevents them to stick together. We use two solutions of PMMA particles with average diameters $\sigma_1$ = 3.77μm and $\sigma_2$ = 4.62μm, as measured by the manufacturer. We write $\sigma = \sigma_1$ =3.77μm, which is taken as the basic length scale in the following discussions. The diameter ratio of the two types of particles is $\sigma_2/\sigma_1 \approx 1.23$. To prepare the systems in the glassy state, we apply a bimodal (binary) mixture of these PMMA spheres to suppress crystallization. The mixture is equimolar with mole fractions $x_1 \approx x_2 \approx 1/2$. Alternatively, to study coexisting glassy and crystalline states, we use a unimodal system containing only the smaller particles, i.e. $x_1 = 1$ and $x_2 = 0$.

In all experiments, particles are immersed in water and confined between the walls of thin transparent glass plates positioned horizontally. The particles fall under gravity onto the lower plate forming quasi-two-dimensional (2D) systems. Digital video microscopy measurements are made using an optical microscope with an oil immersion objective and a CCD camera mounted to the eyepiece. The number of particles within an optical image is typically around 1100. We are able to maintain practically all imaged particles within the depth of focus during the reported periods. Image-processing is performed using particle tracking codes from Ref.(*31*), which extract the trajectories of the centers of all imaged particles. The 2D particle packing fraction $\phi$ is controlled via the initial particle density in the water solution and is measured from microscopic images. For the bimodal samples reported, $\phi$ ranges from 0.70 to 0.80. To ensure equilibrium, we perform production measurements only after samples have been settled for at least 1, 3, and 8 days for $\phi$ = 0.70-0.72, 0.73-0.76 and 0.78-0.80, respectively. Images are recorded at rates of one frame every 1, 2, 3 and 4s for $\phi$ = 0.70, 0.72-0.74, 0.76, and 0.78-0.80, respectively. To capture the slow dynamics at large $\phi$, we record images for durations up to $10^6$ s. This amounts to more than 11 days of continuous imaging. It imposes technical challenges on data storage and particle trajectory analyses, which are overcome by appropriate software selection and minor modifications. Since our particles have relatively large sizes of 3.77μm and 4.62μm, all of them can be automatically identified in nearly all image frames.

A typical image of an experimental bimodal system is shown in Figure S1(a). Figure S1(b) shows the measured probability density function of the particle diameters. Typical particle configurations of experimental and simulated systems with packing fraction of 0.80 are shown in Figure S2.

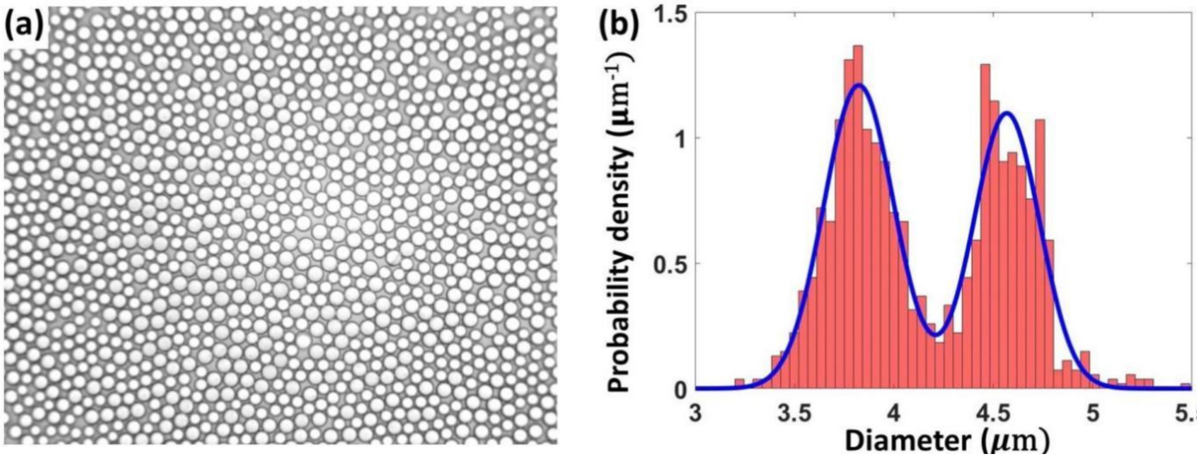


**Figure S1. Experimental Results: (a)** A typical optical image of a bimodal colloidal system. **(b)** Probability density function of particle diameters in the bimodal system. The fitted function (blue curve) is the sum of two Gaussians.

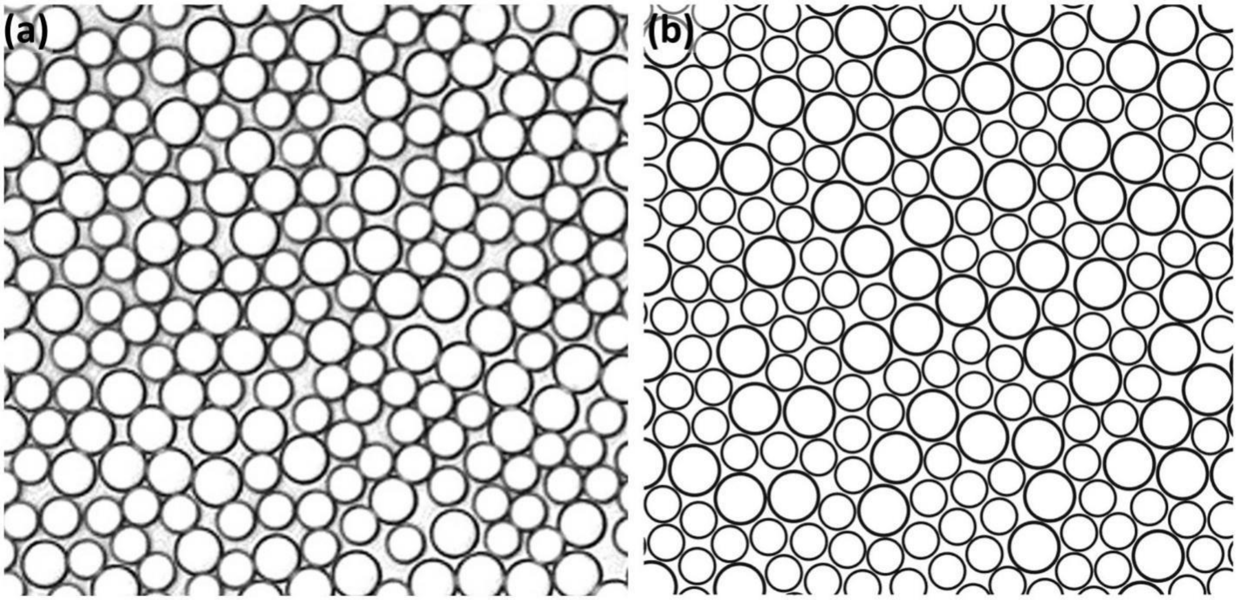


**Figure S2. Experimental and Simulation Results: (a)** An optical image of a bimodal colloidal system at packing fraction $\phi$ = 0.80 and **(b)** a computer simulated bimodal system also at packing fraction $\phi_{MD}$ = 0.80.

### 1.2.Molecular Dynamics Simulations

To verify our experimental observations, we perform molecular dynamics (MD) simulations of glassy colloidal systems in 2D. The systems simulated are the same as those in Ref.(*13*). We adopt non-equimolar binary mixture systems consisting of N hard disks, where N = $64^2$ = 4,096. The mole fractions of small and large disks with diameter of $\sigma_1 = \sigma$ and $\sigma_2 = 1.4\sigma$ are taken as $x_1$ = 2/3 and $x_2$ =1/3 respectively. These conditions have been found to best suppress crystallization (*13*). The disks are placed in a L × L square periodic boundary box, so that the packing fraction

is defined by $\phi_{MD} = N\pi(x_1\sigma_1^2+x_2\sigma_2^2)/4L^2$. In this system, $\phi_{MD}$ is the primary control parameter and it is varied from 0.72 to 0.81. The onset packing fraction between liquid and super-compressed liquids is $\phi_{MD} \approx 0.76$. The basic units of the system are length $\sigma = 1$, particle mass m = 1 and inverse temperature $\beta = 1/k_BT = 1$. The systems are carefully prepared as pure amorphous state even at high $\phi_{MD}$ after long-time equilibrations by efficient event-chain Monte Carlo (ECMC) calculations with up to $O(10^{13})$ collisions (*32*). After equilibration, production runs for extracting particle trajectories are done using Event-Driven MD (EDMD) simulations (*33*).

## 2. Supplementary Results on Glassy Colloidal Systems

### 2.1 Mean Square Displacement (MSD) and Comparing Experiments with Simulations

The measured particle mean square displacement (MSD) for various packing fraction $\phi$ is shown in Figure S3. Very long imaging times have been applied at large $\phi$ to ensure that the MSD have clearly evolved beyond the plateau values. This is important for assessing dynamics dominated by structural relaxations rather than localized vibrations.

Figure S4(a) shows our simulation results on the MSD. Despite exhibiting similar trends as in the experimental results, there are quantitative differences. The simulations show a much stronger dependence of the MSD on $\phi_{MD}$ with a more dramatic slowdown as $\phi_{MD}$ increases. The discrepancies may mainly be due to the effectively softer nature of the experimental particles resulting from the quasi-2D setup, in contrast to the genuine 2D systems of perfectly hard particles. Specifically, larger particles stand taller than smaller ones as they all rest under gravity on the lower glass plate. They may be momentarily squeezed slightly upward in crowded situations, and this creates additional free volumes for particles to move around. The kinetic arrest may thus be more stretched out with respect to $\phi_{MD}$. The finite rigidity of the experimental particles may also contribute to the softness. There are also other factors forbidding the direct comparison of $\phi$ and $\phi_{MD}$ in experiments and simulations. These include the slightly different particle radius distributions and mode fractions of the large versus small particles, which have been independently chosen to best suppress crystallization in the respective systems.

To enable qualitative comparisons between experiments and simulations, we apply an empirical multiplication factor of 0.025s to map the simulation time unit to physical time. Then, the experimental and simulation results follow a consistent trend as shown in Figure S4(b). For each packing fraction, we next find the time $t_{0.2}$ at which the MSD = $0.2\sigma^2$. A plot of $t_{0.2}$ against $\phi$ and $\phi_{MD}$ is shown in Figure S4(c). The experimental data of $t_{0.2}$ is fitted to a linear function in the semi-log scale as a first approximation. Finally, for each simulated packing fraction $\phi_{MD}$, the corresponding value of $\phi$ is chosen as the one which provides the same value of $t_{0.2}$ according to the fitted line. Figure S4(d) plots the mapped value of $\phi$ as a function of $\phi_{MD}$ hence obtained.

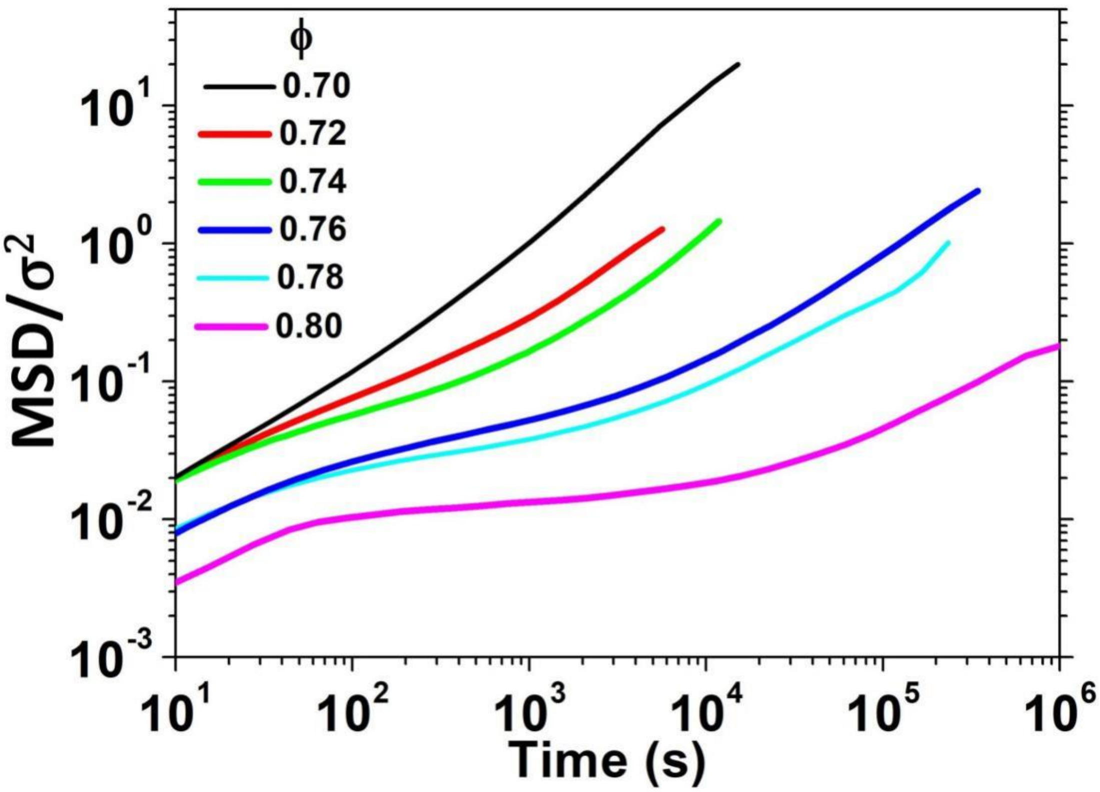


**Figure S3. Experimental Results:** Particle mean square displacement (MSD) against time for various packing fraction $\phi$.

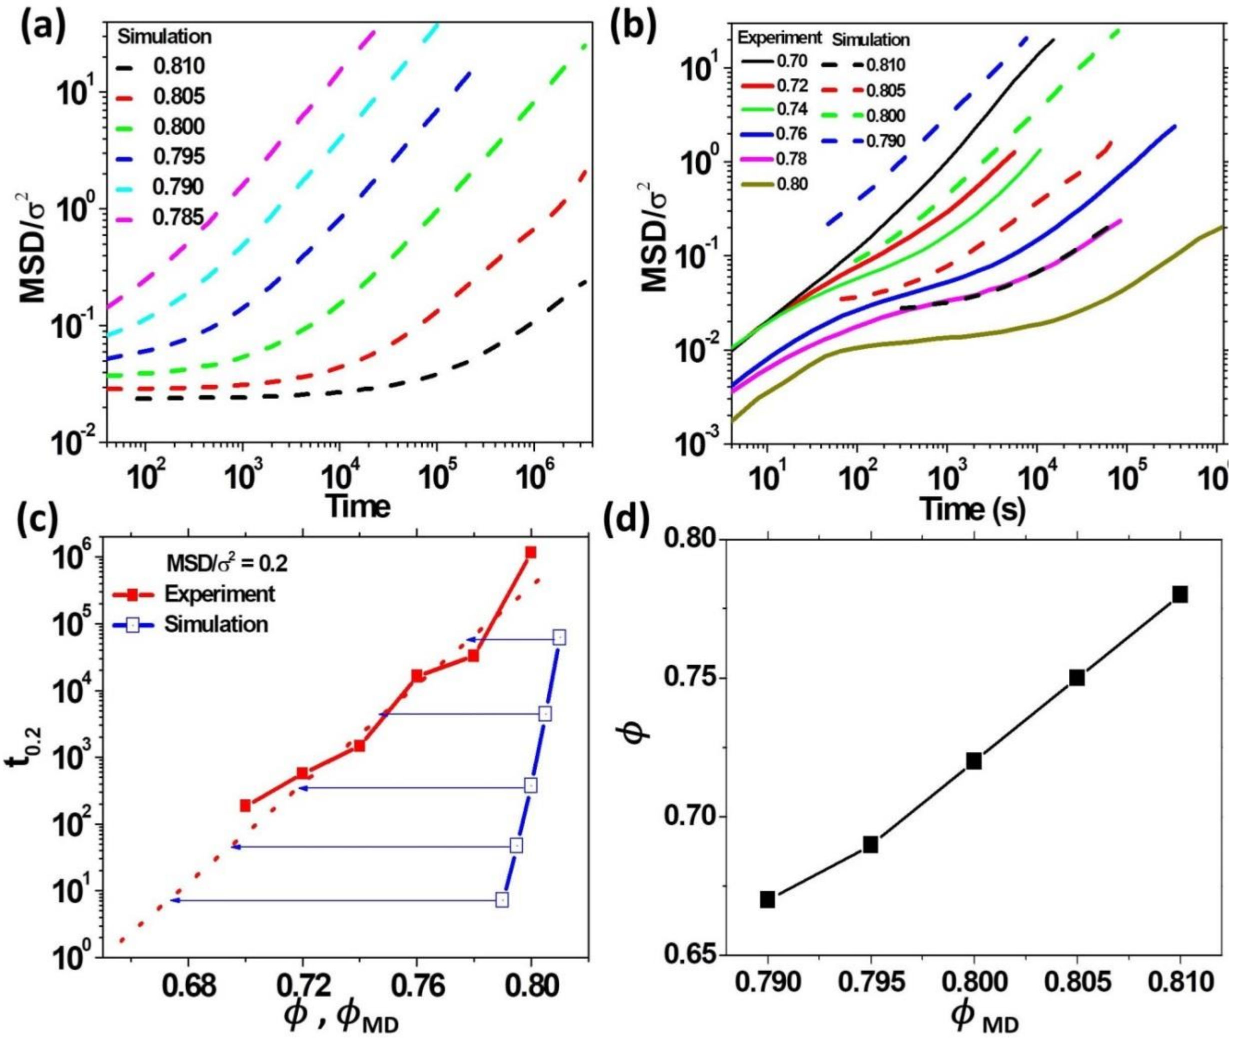


**Figure S4. Experimental and Simulation Results: (a)** MSD against time from simulations. **(b)** MSD against time from experiments and simulations. **(c)** A plot of $t_{0.2}$ versus $\phi$ and $\phi_{\mathrm{MD}}$ from experiments and simulations, where $t_{0.2}$ is the time to attain a MSD of $0.2\sigma^2$. The blue arrows show the mapping of $\phi_{\mathrm{MD}}$ to $\phi$. Note that time in simulations in (b) and (c) have been converted to physical units using an empirical factor of 0.025s. **(d)** Mapping of packing fraction from $\phi_{\mathrm{MD}}$ to $\phi$.

## 2.2. Particle Displacement Distribution, Particle Hops and Coarse-grained Trajectories

We now study the displacement $\Delta r_i^c = |\vec{r}_i^c(t) - \vec{r}_i^c(0)|$ of each particle over time $t$ based on instantaneous particle position $\vec{r}_i^c(t)$. Figure S5 shows the probability density function P($\Delta r/\sigma$) of the normalized displacement $\Delta r/\sigma$ averaged over particles and different definitions of time 0. Note that P($\Delta r/\sigma$) is proportional to the van Hove correlation function. At small $t$, we observe a single-peaked function. As $t$ increases, a secondary peak emerges at $\Delta r \approx 1.2\sigma$, representing activated hopping events. The peaks are separated by a dip at $\Delta r \approx 0.8\sigma$, which we take as the threshold of hopping. As shown in Figure S6, simulations show very similar behaviors.

The detailed dynamics during a particle hop can be illustrated by the normalized displacement $\Delta r/\sigma$ plotted against time $t$ during a hopping event and the hopping dynamics at $\phi$ = 0.80 is shown in Figure S7. The step-like increase in $\Delta r/\sigma$ signifies a hop. The sudden rise takes a time, called the instanton time (12), to complete, which is about 200s in this example. Figure S8 shows a similar result from simulations at $\phi_{\mathrm{MD}}$ = 0.810, in which the instanton time is about 2000.
Further analyses of particle dynamics are based on coarse-grained particle positions defined by $\vec{r}_i^c(t) = \langle \vec{r}_i(t') \rangle_{t' \epsilon [t, t+\Delta t_c]}$, as already explained in the main text. Figure S9(a)-(d) show coarse-grained particle trajectories for the example of $\phi$ = 0.76. Each trajectory is generated by joining time sequences of coarse-grained positions $\vec{r}_i^c(t)$ at $t$ = 0, $\Delta t_c$, $2\Delta t_c$, ..., $T_{traj}$. For small $T_{traj}$ and $\Delta t_{c,}$ considered in Figure S9(a), particles show small displacements in general. As both $T_{traj}$ and $\Delta t_c$ increase in Figures S9(b)-(d), many of the small displacements are increasingly averaged out, but some others reach lengths of order σ and represent string-like hopping motions. An extraordinarily high mobility contrast between particles is observed in Figure S9(d), indicating that hopping motions dominate the dynamics.

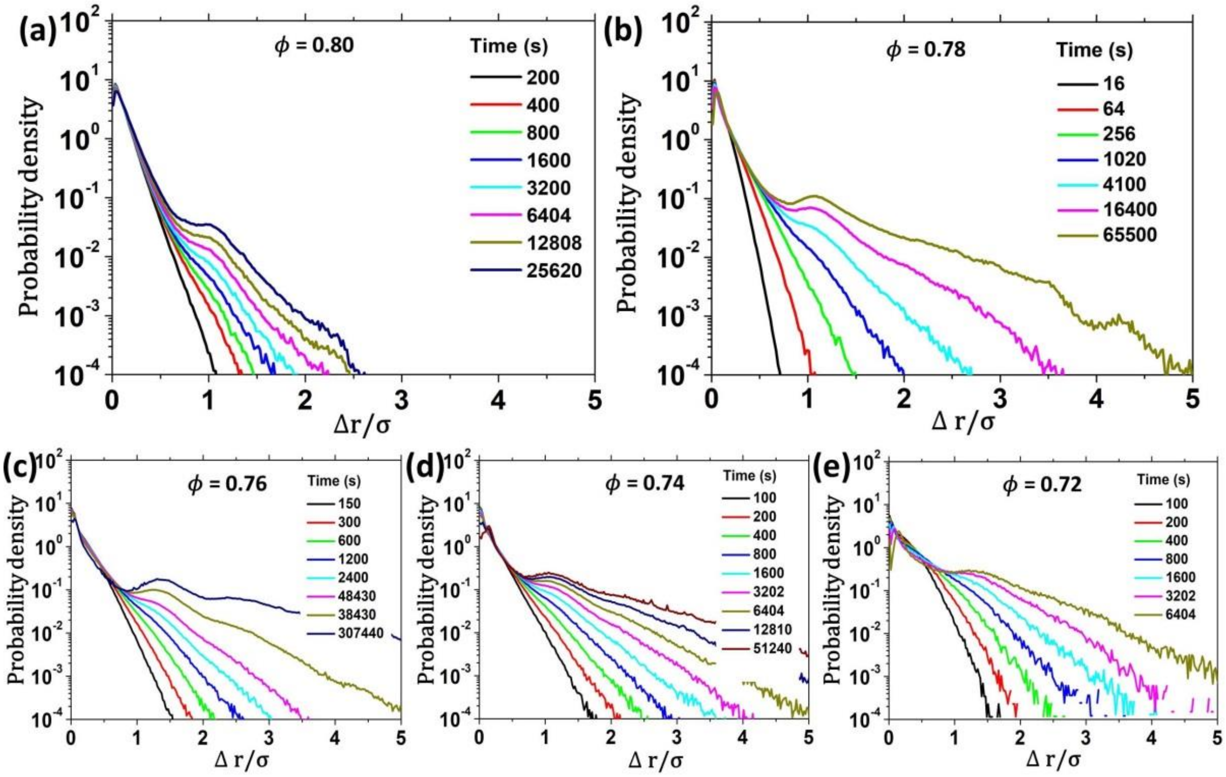


**Figure S5. Experimental Results:** Probability density function of particle displacement $\Delta r$ in unit of σ based on instantaneous particle positions for packing fraction **(a)** $\phi$ = 0.80, **(b)** 0.78, **(c)** 0.76, **(d)** 0.74, and **(e)** 0.72. In each case, a peak emerges at $\Delta r \approx 1.2\sigma$ and an accompanying dip appears at $\Delta r \approx 0.8\sigma$ as time t increases.

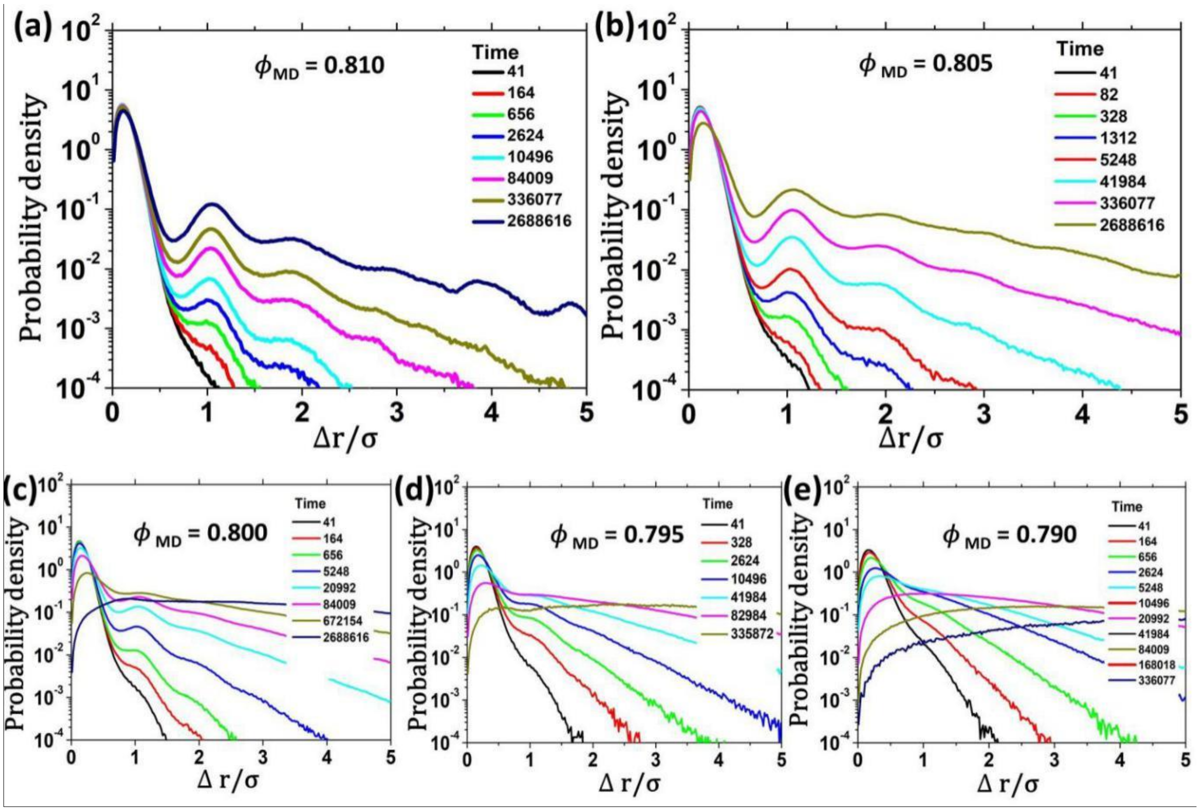


**Figure S6. Simulation Results:** Probability density function of particle displacement $\Delta r$ in unit of $\boldsymbol{\sigma}$ based on instantaneous particle positions for packing fraction **(a)** $\phi_{\mathrm{MD}}$ = 0.810, **(b)** 0.805, **(c)** 0.800, **(d)** 0.795, and **(d)** 0.790.

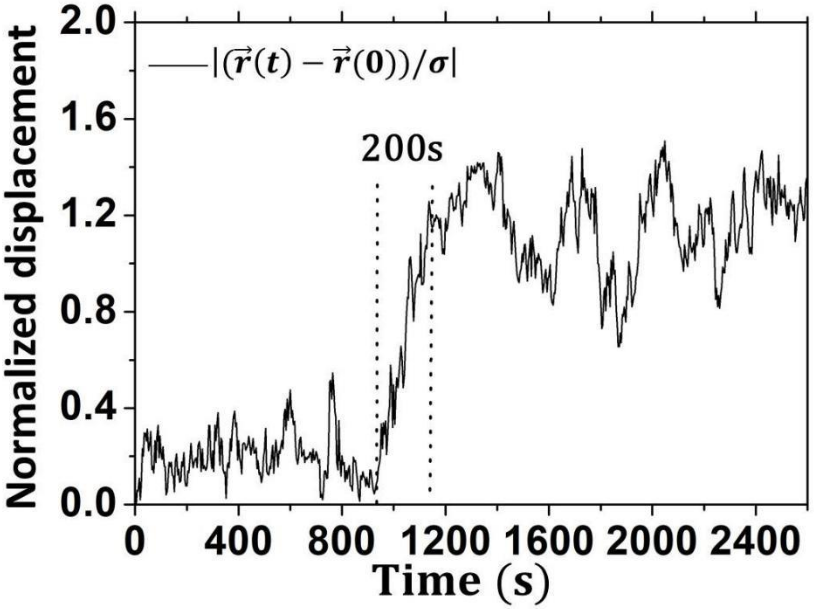


**Figure S7. Experimental Results:** Particle displacement $\Delta r$ in unit of σ against time t based on instantaneous particle positions during a hopping event for $\phi$ = 0.80. The instanton time is about 200s. The particle vibrates around metastable states before and after the hop.

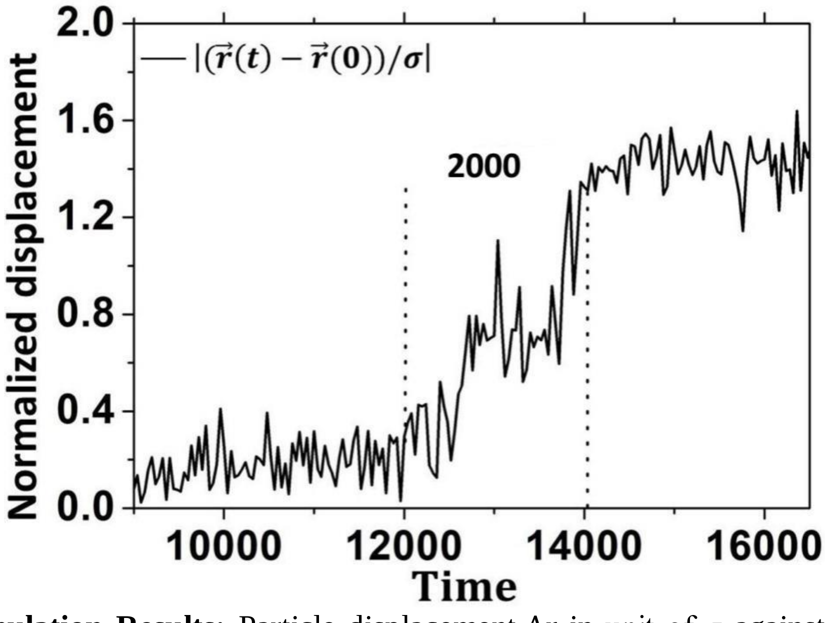


**Figure S8. Simulation Results:** Particle displacement $\Delta r$ in unit of σ against time t based on instantaneous particle positions during a hopping event for $\phi_{MD}$ = 0.810. The instanton time is about 2000.

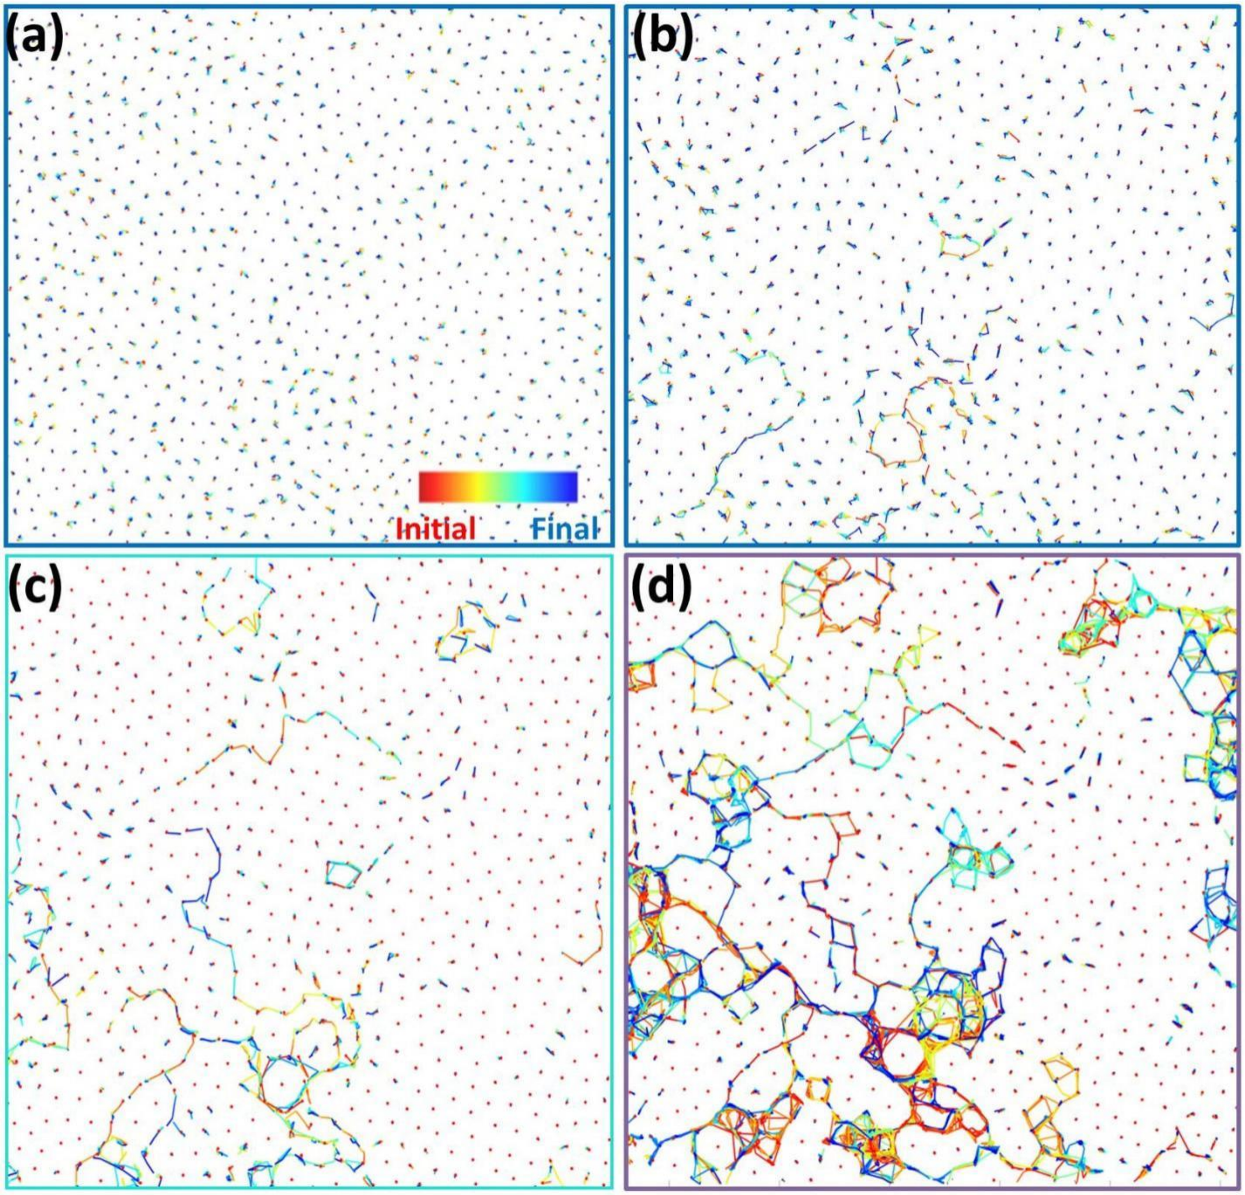


**Figure S9. Experimental Results:** Time-colored coarse-grained particle trajectories at $\phi$ = 0.76. Each trajectory is represented by line segments joining consecutive coarse-grained particle positions. We take **(a)** $T_{traj}$ = 600 s, $\Delta t_c$ = 8s **(b)** $T_{traj}$ = 1200s, $\Delta t_c$ = 120s, **(c)** $T_{traj}$ = 18000s, $\Delta t_c$ = 900s and **(d)** $T_{traj}$ = 350000s, $\Delta t_c$ = 1750s, where $T_{traj}$ is the time duration covered by a whole trajectory and $\Delta t_c$ is the time interval during which a coarse-grained particle position is averaged over. Line segments are colored according to time from red to blue, following Figure 1(a) of the main text. Initial particle positions are denoted by red dots.

## 2.3. String-like motions and quasi-voids

We have illustrated string-like motions and quasi-void dynamics in Figs. 1 and 2 in the main text based on particle trajectories and configurations extracted from optical images using particle identification and tracking software. To confirm that our conclusions are not artifacts of these sophisticated analysis methods, we now examine the optical images more directly using a simple image compositing approach.

Figure S10(a)-(b) shows optical images of our experimental colloidal system before and after the string-like motion in Fig. 1(b)-(c) in the main text. We have colored those particles related to the motion for easier identification. Free volumes can be understood as spaces available throughout the system for inserting a new particle (*34*). The fragmented free volumes constituting the quasi-void being transported are illustrated as the blue areas. The particle configurations observed in the optical images in Fig. S10(a)-(b) is fully consistent with the computer regenerated images in Fig. 1(b)-(c) based on tracked particle positions.

Figure S10(c) shows a composite optical image clearly illustrating the particle movements. It is essentially a time-averaged optical image of the initial configuration put on top of a time-averaged image of the final configuration, after the latter has been converted to cyan. Only simple pixel-wise image processing operations are used. Specifically, the initial (final) image is obtained by averaging over the red-green-blue (RGB) values of 8 time-consecutive images before (after) the string-like motion. Let $(r^I, g^I, b^I)$ and $(r^F, g^F, b^F)$ be the RGB values of a pixel in the initial and final averaged images respectively. The corresponding pixel in Fig. S10(c) is then assigned an RGB value of $\max\{ (r^I, g^I, b^I), (0, g^F, b^F) \}$. The maximum operation ensures that a white pixel dominate over a colored one of the same intensity and hence provides the perception of being on top. Similarly, Fig. S10(d) shows the final image on top of the initial one which is converted to red. Technically, the pixel value is calculated by $\max\{ (r^I, 0, 0), (r^F, g^F, b^F) \}$.

We reproduce Fig. S10(c)-(d) in Fig. S10(e)-(f) with added annotations, including blue arrows showing the displacements of the relevant particles. In Fig. S10(e), a region close to the string tail, as defined in the main text, is illustrated by a yellow dotted line. The region initially holds four particles. During the string-like motion, a particle (the big purple particle in Fig. S10(a)) moves by a distance comparable to its diameter and enters the region nearly completely. The region thus finally holds five particles. Since we consider a high packing fraction, the region must initially possess a higher than average amount of free volumes, which can clearly be observed in Figs. S10(a), (c) and (e). We have defined the quasi-void as the free volumes which allow for this extra particle in the region and are shaded schematically in blue in Fig. S10(a). Similarly, from Fig. S10(f), a particle (the orange particle in Fig. S10(a)) exits the region marked by the dotted yellow line. The region originally holding four particles is then left with only three. Equivalently, one quasi-void resides in the region in the final configuration as indicated by the blue areas in Fig. S10(b).

As exemplified in Fig. S10, a string-like motion in general involves a number of particles internal to the string with displacements close to the average particle diameter (i.e. 1.12σ in our colloidal system) and displaces the preceding particles nearly completely. In addition, there is also a tail region which loses a quasi-void and a head region which gains a quasi-void.

We adopt explicit rules to define the free-volume fragments in a quasi-void, based on a particle push-off process. Figure S11 illustrates the rules schematically for the simplified case of a one-dimensional arrangement of particles with a uniform radius σ close to the string head. In this definition, the center of the quasi-void is located at the center of the final position of the particle at the string head. The effective quasi-void area is the invaded area of the string head, after other particles are pushed-off. It equals about 90% of the area of the particle at the string head, which may be a large or small particle. The free-volume gain from pushing off a particle dictates the geometries of the free-volume fragments to be iteratively included in the quasi-void.

It can be straightforwardly generalized to 2D in which the fragments are not only translated but also rotated by the angle between the displacement vectors of the pushing and pushed particles. In addition, a linear sequence of pushing off may become a branched process. With the above definition, the quasi-void can be objectively identified.

Similar dynamics is observed in our MD simulations. Figure S12 shows a typical string-like motion at $\phi_{\mathrm{MD}}$ = 0.810, which is the highest packing fraction simulated in this work. We have also illustrated schematically the fragmented free volumes of a quasi-void which are transported by the string-like motion from one end to the other end of the string.

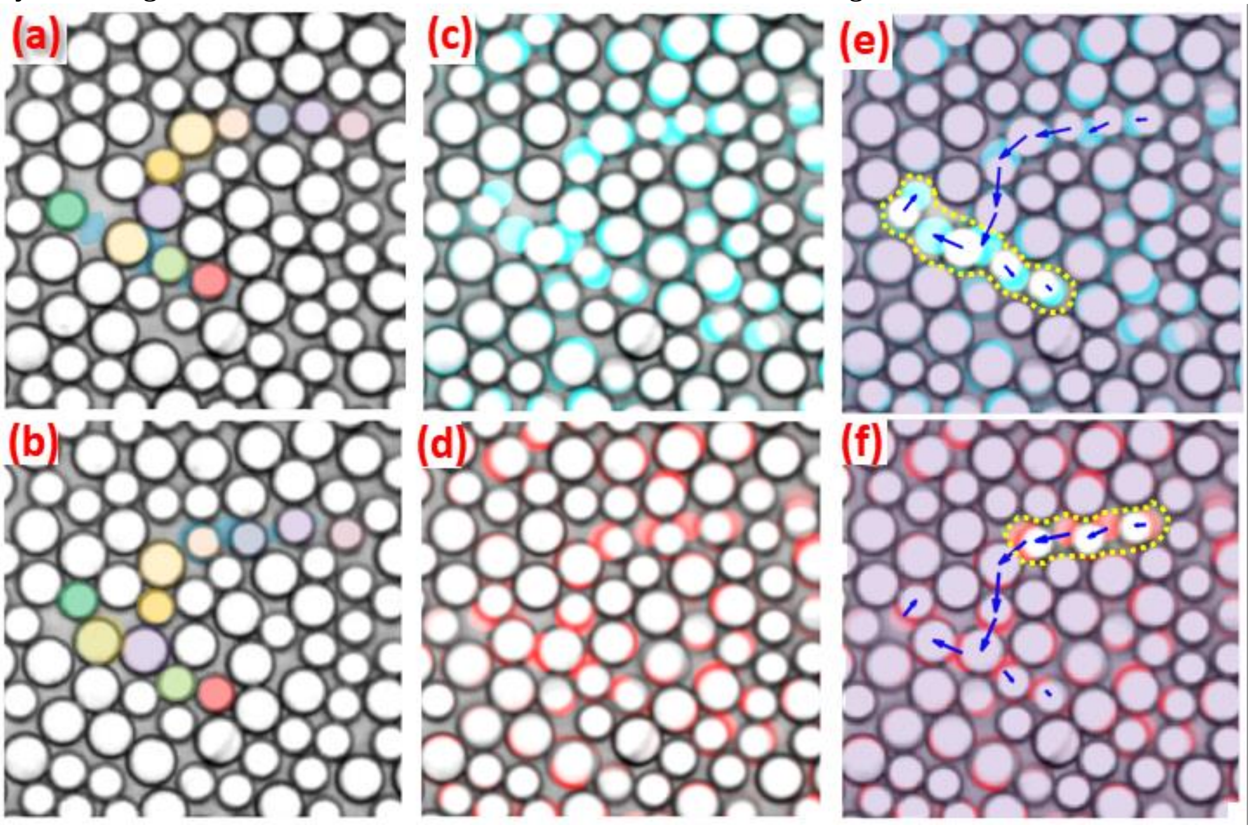


**Figure S10. Experimental results: (a)-(b)** Optical images showing initial (a) and final (b) particle configurations before and after a string-like motion. The same motion is also illustrated in the computer regenerated images in Figure 1(b) and (c) in the main text. Particles involved in the motion are colored for easier identification. The fragmented free volumes constituting the quasi-void being transported are illustrated as blue areas. **(c)** A composite optical image with initial particle configuration (white) shown ‘on top of’ the final configuration (blue). The initial

and final images used are each averaged over 8 raw images to suppress effects of vibrations. **(d)** A composite optical image similar to (c) with final particle configurations (white) shown 'on top of' the initial configuration. **(e)** The same composite image in (c). A region (yellow dotted line) initially contains 4 particles and one quasi-void but finally holds 5 particles. Displacements of particles related to the string-like motion are illustrated by blue arrows. **(f)** The same composite image in (d) illustrating a region (yellow dotted line) holding 4 particles initially in contrast to 3 particles and one quasi-void finally.

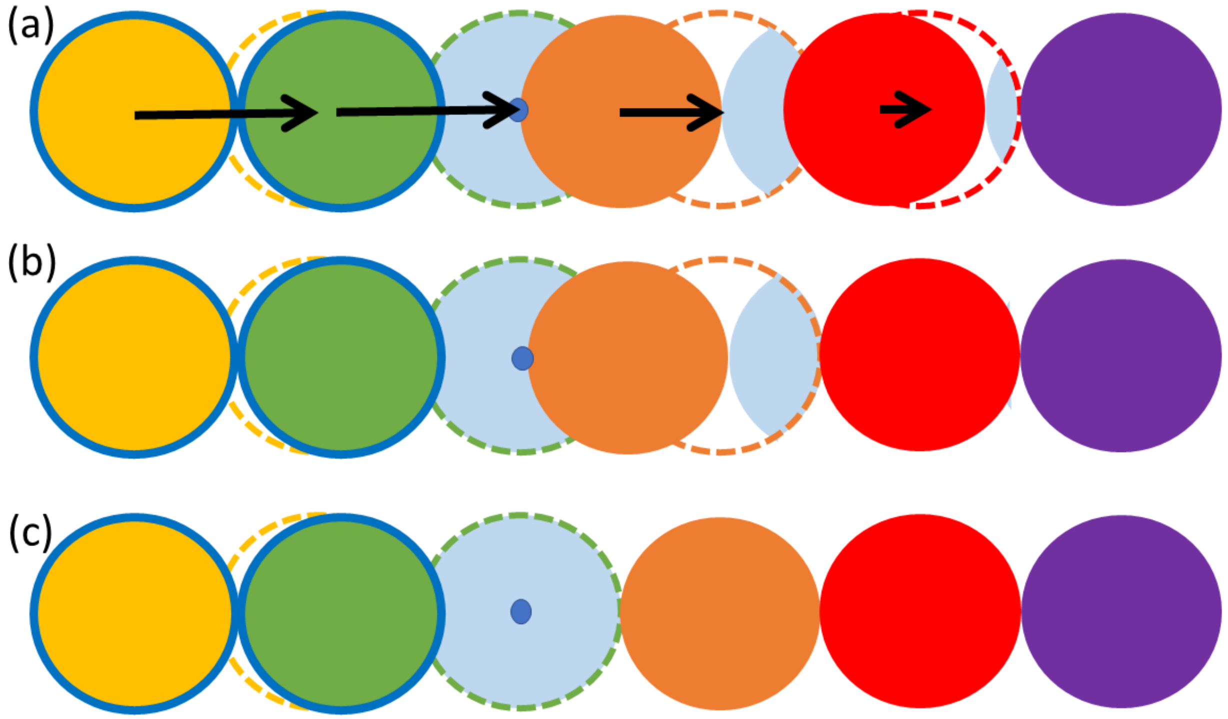


**Figure S11. (a)** Schematic diagram of initial (solid spheres) and final (open spheres) configurations of particles close to the head of a string-like motion. Their displacements are indicated as black arrows. The green and yellow particles has large displacements ( $> 0.8\sigma$) and take part in a string-like motion, which also induces smaller displacements of the orange and red particles. The green particle located at the invading end of the string is defined as the string head. The quasi-void transported by the string is defined as consisting of three free-volume fragments (blue areas). Its position is defined for simplicity as the center of the final position of the string head (blue dot), which may or may not be occupied by a particle initially. The string head is able to move to its final position because particles in front (orange and red) are sequentially pushed off, a process transporting and effectively reassembling the required free volume fragments. **(b)** To schematically reassemble the fragments, the right fragment is first transported by the movement of the red particle to combine with the middle fragment. **(b)** The combined fragment is further transported by the movement of the orange particle to combine with the main fragment on the left. **(c)** The fragments have been constructed so that the reassembled free volume coincides with the invaded volume by the string head. Note however that particles in general move simultaneously and configurations in **(b)** and **(c)** are for illustration only.

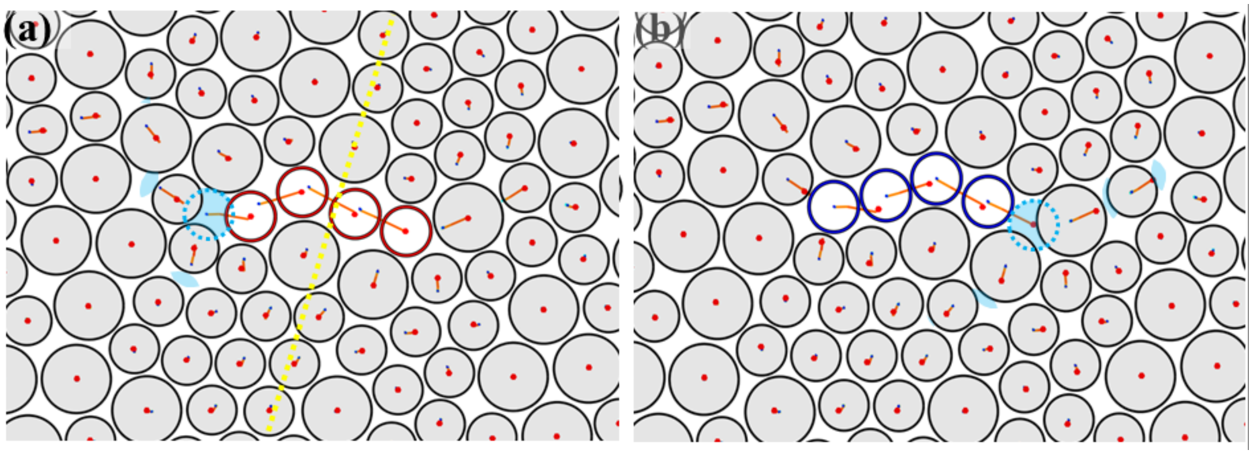


**Figure S12. Simulation Results: (a)** and **(b)** Coarse-grained trajectories for duration $T_{traj}$ = 20 showing a typical string-like particle hopping motion at packing fraction $\phi_{MD} = 0.810$. Particle configurations at the beginning **(a)** and the end **(b)** of the period are also shown. A quasi-void consisting of fragmented free volumes (blue areas) is transported by the string across a line of otherwise nearly stationary particles (yellow dotted line). Note that the blue dotted circles show the final position of the particle at the string tail in (a) and the initial position of the particle at the string head in (b).

## 2.4. Displacement Correlation and Particle Back-and-forth Hopping Motions

From coarse-grained particle trajectories at large $\phi$, we observe particle hops in a background of nearly stationary particles. This is in sharp contrast to typical collective flow in non-glassy liquids in which particles tend to move with stronger local correlations. To quantify this high mobility contrast in the glassy phase, we have defined a displacement correlation $Y$ in Eq. (1) in the main text which is reproduced here as:

$$Y = \left\langle min\{\Delta r_j\}_{j\in\Omega_i}/\Delta r_i\right\rangle_{i\in\Omega_{hop}}.$$

In this formula, $\Delta r_i = |\vec{r}_i^c(t+\delta t) - \vec{r}_i^c(t)|$ is the coarse-grained displacement of particle i over a duration $\delta t$ at time t. We only consider particle i in the set $\Omega_{hop}$ of hopped particles, satisfying $\Delta r_i > 0.8\sigma$ with the threshold 0.8σ corresponding to a dip in the van Hove correlation function (see Figure S5). We then examine the set $\Omega_i$ of nearest neighbors of particle i, which is defined as its 6 nearest particles based on coarse-grained particle positions at time t. The correlation $Y$ is the minimum value of the coarse-grained displacements $\Delta r_j$ of these neighboring particles, after being normalized by $\Delta r_i$. We have averaged $Y$ over all hopping particles i and time t. Under this definition, string-like motions should contribute little to $Y$ because not all 6 neighboring particles participate in the string in general. Hence, $Y$ measures mainly the magnitude of the collective flow component of the dynamics.

Figure S13(a) shows the results of $Y$ against $\phi$. Coarsened particle positions $\vec{r}_i^c$ are calculated by averaging instantaneous positions over an averaging time $t_c$ = 10, 20, 30 and 40s for $\phi$ = 0.70, 0.72-0.74, 0.76 and 0.78-0.80, respectively, which correspond to 10 recorded image frames in all cases. We have also taken $\delta t \approx$ 400s for all values of $\phi$. This choice of $\delta t$ is shorter than a typical

waiting time of a particle hop so that double hops within the duration are few. In addition, it is longer than the instanton time (see Sec. 2.2 in SI), which is the typical duration of the course of a hopping event. To illustrate particle motions under these coarsening parameters, Figure S14 shows examples of particle trajectories under these coarsening conditions. Similarly, Figure S13(b) shows results on Y from simulations, where we have taken $\delta t$ = 67240 and $\Delta t_c$ = 1681 for all values of $\phi_{MD}$. Corresponding coarse-grained trajectories from simulations are shown in Figure S15.

Figures S13(a-b) both show a similar trend of $Y$ decreasing with $\phi$. For a quantitative comparison, we reparametrize $\phi_{MD}$ to $\phi$ based on the particle MSD measurements explained in Sec. 2.1 in SI. The results are shown in Figure 4(a) in the main text. The good quantitative agreement then obtained is non-trivial and shows that the simulations indeed closely model the experiments. The monotonic decrease of Y towards 0 in Figure 4(a) shows the diminishing role of collective flow as $\phi$ increases. This supports the study of glassy dynamics based solely on hopping motions.

To quantify back-and-forth particle hops, we calculate the returning and escaping probabilities $P_{ret}$ and $P_{esc}$ of hopped particles. Using the same definitions of particle hops above, we monitor the further motions of particle $i$ which has hopped during the period from $t$ to $t$+$\delta t$. We examine its coarse-grained position $\vec{r}_i^c(t')$ at later times $t'$= $t$+$\delta t$+$n\Delta t_c$ (n = 1, 2, ...) up to $t$+$\delta t$+$\tau_{max}$. If it first returns to its original position, i.e. $|\vec{r}_i^c(t') - \vec{r}_i^c(t)| < 0.4\sigma$, the motion is referred to as a returning hop. Alternatively, if it first hops again to a third position, i.e. $|\vec{r}_i^c(t') - \vec{r}_i^c(t + \delta t)| > 0.8\sigma$, we classify it as an escaping hop. Otherwise, the particle is deemed stationary. The particle returning and escaping probabilities $P_{ret}$ and $P_{esc}$ are hence calculated.

Figure S16(a-b) shows the results on $P_{ret}$ and $P_{esc}$ for experiments and simulations. We have taken the same values of $t_c$ and $\delta t$ given above for the calculation of $Y$. For the experiments, we put $\tau_{max}$ = 1000s, 6000s, 90000s, 96000s and 360000s for $\phi$ = 0.70-0.72, 0.74, 0.76, 0.78 and 0.80 respectively. For the simulations, $\tau_{max}$ = 1000, 2000, 6000 and 7000 and 8000 for $\phi_{MD}$ = 0.785-0.790, 0.795, 0.800, 0.805 and 0.810 respectively. These values of $\tau_{max}$ are large enough so that particles have returned or escaped in most cases resulting at $P_{ret}$ + $P_{esc}$ > 90%.

Similar to the study of Y above, experimental and simulation results on $P_{ret}$ and $P_{esc}$ show consistent trends. Again, after reparametrizing $\phi_{MD}$ to $\phi$ based on the particle MSD, a good quantitative agreement is obtained as shown in Figure 4(b) in the main text. We have obtained from experiments a very high probability of $P_{ret} \approx 0.80$ for returning events, which appears to further increase towards 1 as $\phi$ increases. This shows the quantitative, and possibly, even qualitative importance of back-and-forth particle hopping motions. Such motions are observable directly from particle trajectories as shown in Figure S17.

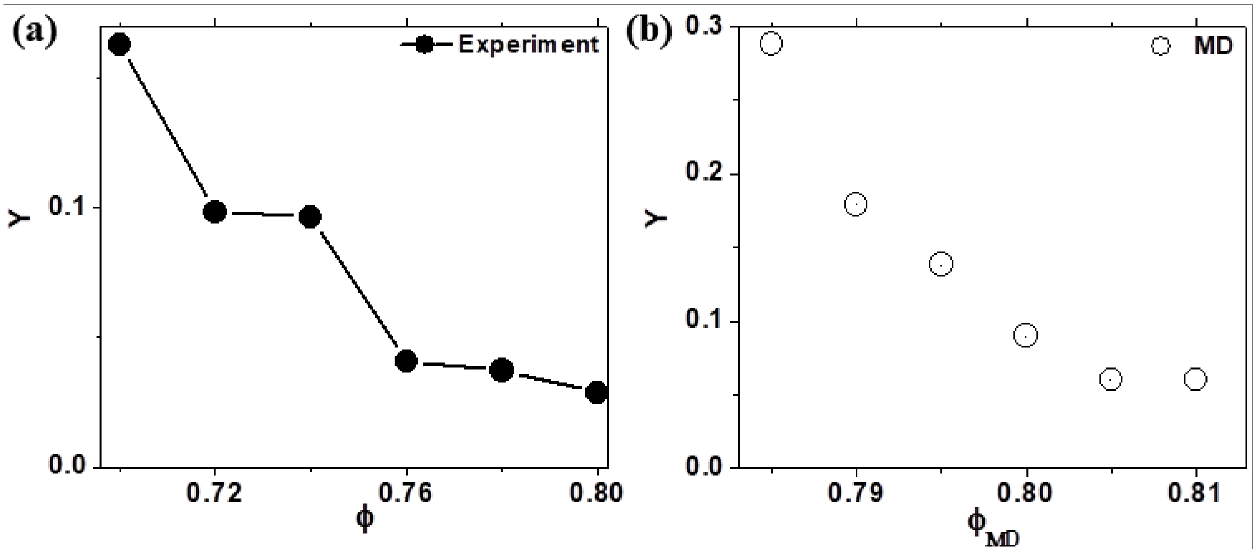


**Figure S13. Experimental and Simulation Results:** Displacement correlation Y against packing fraction $\phi$ and $\phi_{\mathrm{MD}}$ from **(a)** experiments and **(b)** simulations.

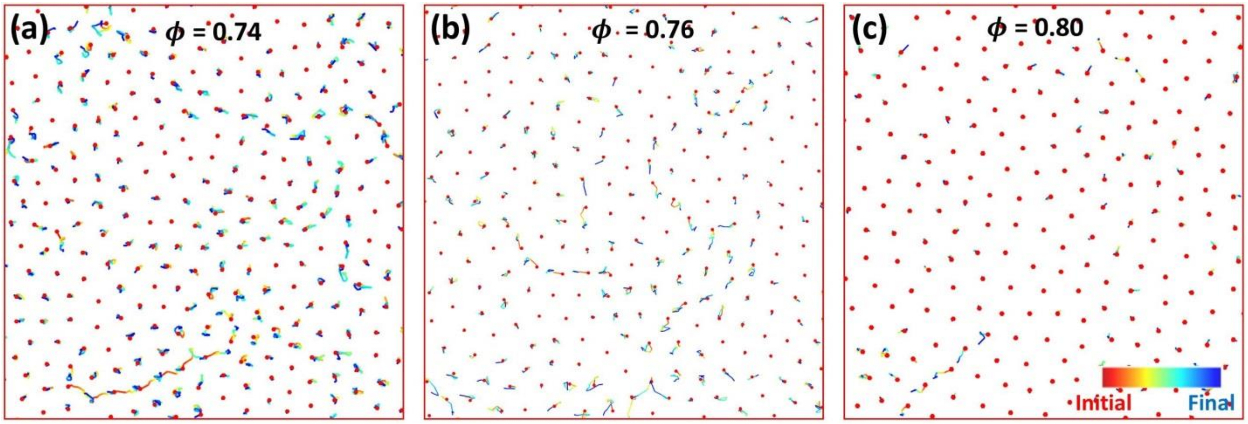


**Figure S14. Experimental Results:** Typical particle trajectories for coarsening parameters $\delta t$ and $\Delta t_{\mathrm{c}}$ used in calculating Y, $P_{ret}$ and $P_{esc}$ for $\phi$ = **(a)** 0.74, **(b)** 0.76, and **(c)** 0.80.

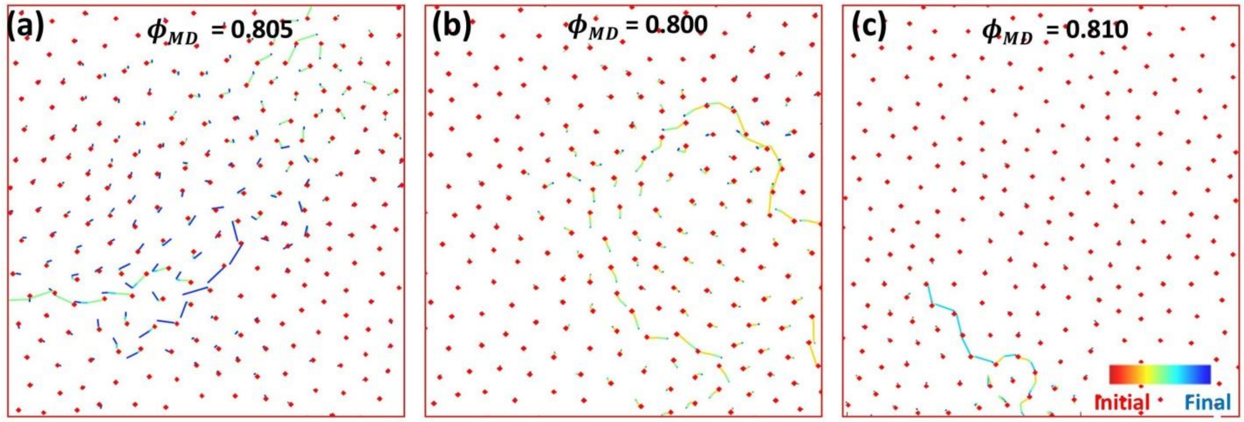


**Figure S15. Simulation Results:** Typical particle trajectories for coarsening parameters $\delta t$ and $\Delta t_{\mathrm{c}}$ used in calculating Y, $P_{ret}$ and $P_{esc}$ for $\phi_{\mathrm{MD}}$ = (**a**) 0.800, (**b**) 0.805, and (**c**) 0.810.

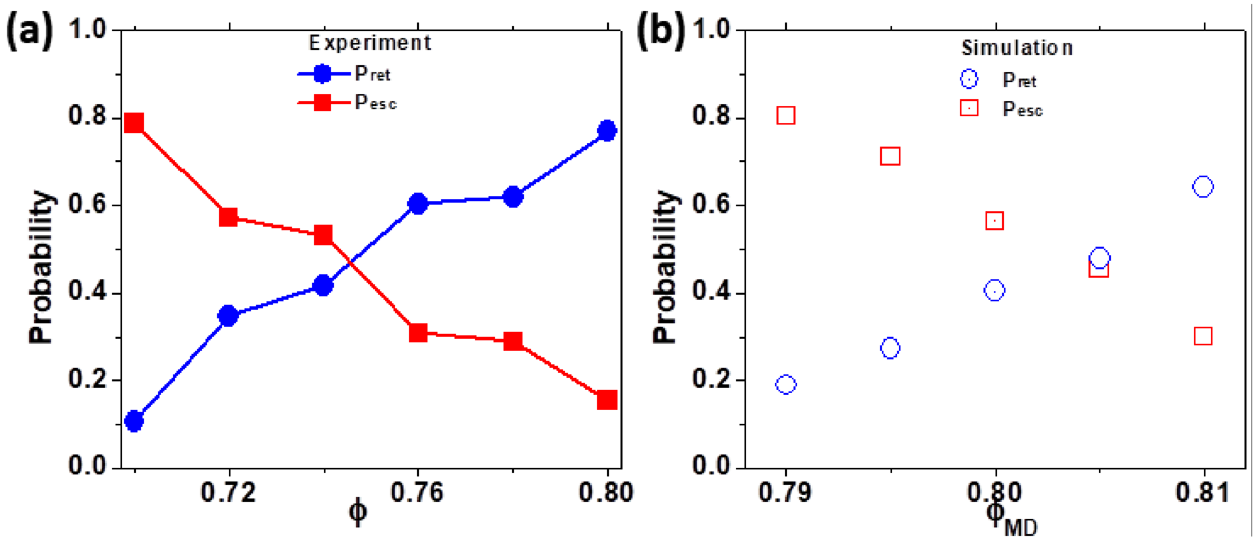


**Figure S16. Experimental and Simulation Results:** Returning and escaping probabilities $P_{ret}$ and $P_{esc}$ of hopped particles against packing fraction $\phi$ and $\phi_{\mathrm{MD}}$ from **(a)** experiments and **(b)** simulations.

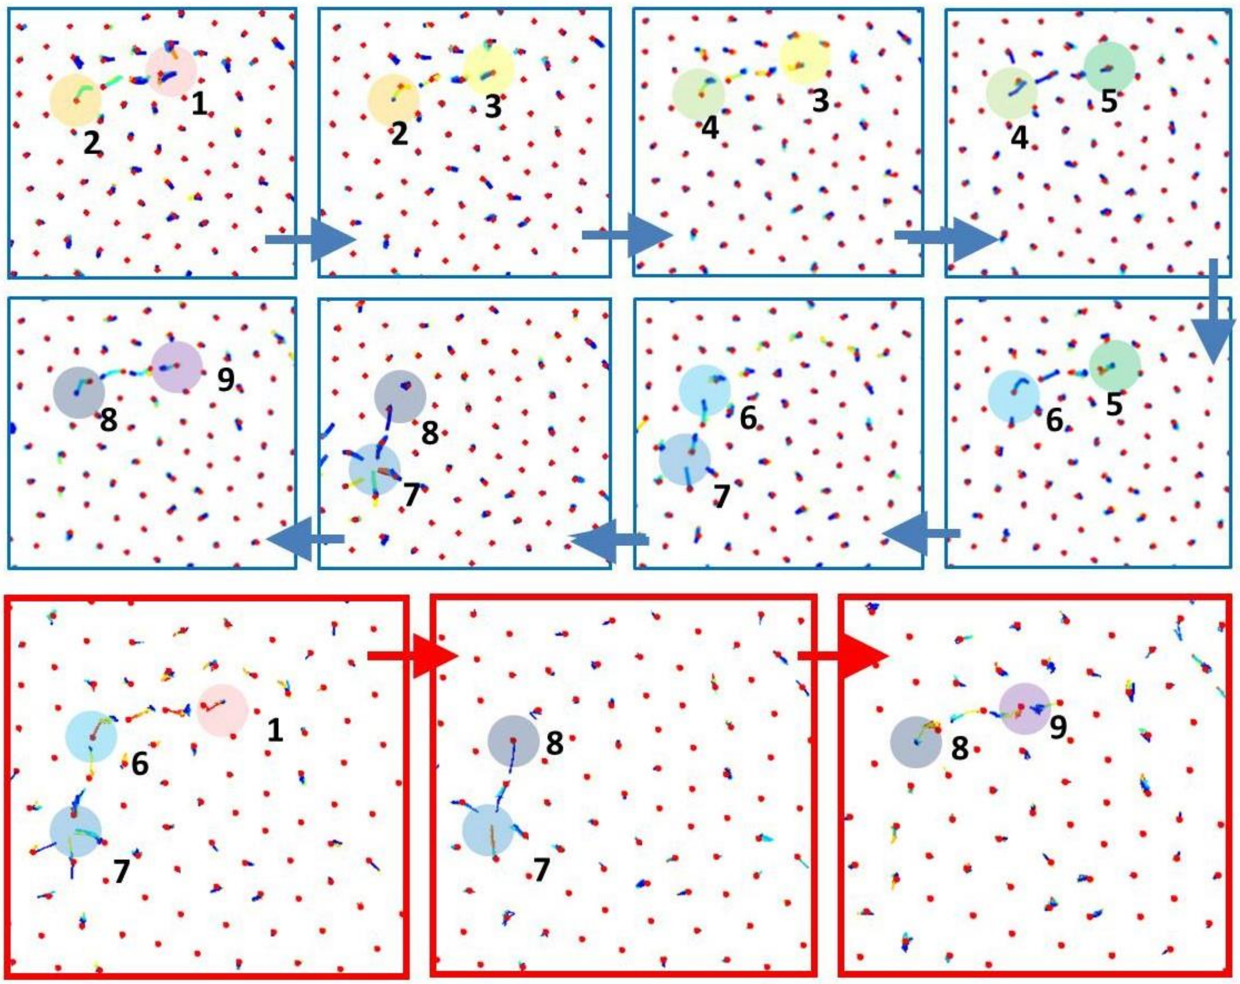

**Figure S17. Experimental Results:** Blue boxes: Consecutive time sequence of coarse-grained trajectories at $\phi$ = 0.80. Numbered circles mark initial and final positions of a quasi-void. Many back-and-forth motions are observed. Red boxes: Consecutive time sequence of the same motions as in the blue boxes but at longer coarsening times. Some back-and-forth motions are hidden by the further coarsening.

### 2.5. String-like motions in mobile clusters

For each value of $\phi$, we show in Figure S18 particle trajectories over time $T_{traj}$ so that particle MSD ≈ 0.2$\sigma^2$. We identify the mobile particle group as the set of particles with coarse-grained displacements $\Delta r_i^c = \left|\vec{r}_i^c(T_{traj}) - \vec{r}_i^c(0)\right|$ within the top 15% among all particles. Particles in the mobile group are represented by solid circles in Figure S18. Note that some particles exhibiting back-and-forth motions and having returned to the original positions are not considered mobile under this widely used definition. We further classify the mobile particles as core-like and string-like depending on the local neighboring conditions of the mobile particles following Ref (*7*). They are colored as red and blue respectively in Figure S18. Our results show a clear trend of a crossover from predominantly string-like to predominantly core-like mobile domains, in full agreement with the observation in Ref(*7*). In fact, an analogous crossover of the geometries of mobile particles is also observable from a lattice model of glass (see Figure. 7 of Ref(*20*)).

We have shown in Figure 3 of the main text particle trajectories in a cluster of core-like particles. Detailed trajectories show that particle motions are indeed composed of two sequences of string-like motions induced by two quasi-voids. As further examples, detailed dynamics in three core-like clusters Figure S18(c) are illustrated in Figures S19-S21. They similarly show sequences of string-like motions. Similarly, Figures S22 shows trajectories in a core-like cluster from simulations broken down into sequences of string-like motions.

All these examples show that particle dynamics are dominated by string-like motions induced by quasi-voids even at a large $\phi$ for both string-like and core-like clusters, despite apparently different cluster geometries. The compact core-like geometries in fact result from the increased dynamic heterogeneity at large $\phi$, meaning that particle hops recur again and again at highly localized regions so that strings superimpose each other to form compact clusters. The string dominated dynamics are otherwise similar to those in string-like clusters and at smaller values of $\phi$. We have studied trajectories covering durations $T_{traj}$ at which the MSD ≈ 0.2$\sigma^2$. We take $T_{traj}$ = 360s, 15000s and 1000000s for $\phi$ = 0.72, 0.76 and 0.80 respectively. The top 15% mobile particles are found to have displacements $\Delta r_i$ beyond 0.33 σ, 0.27 σ and 0.42 σ respectively, which should be large enough to exclude most vibrations, despite being smaller than our threshold 0.8σ of hopping used above. We emphasize that these conditions are important to observe true glassy dynamics as they ensure the dominant role of structure relaxations as opposed to vibrations.

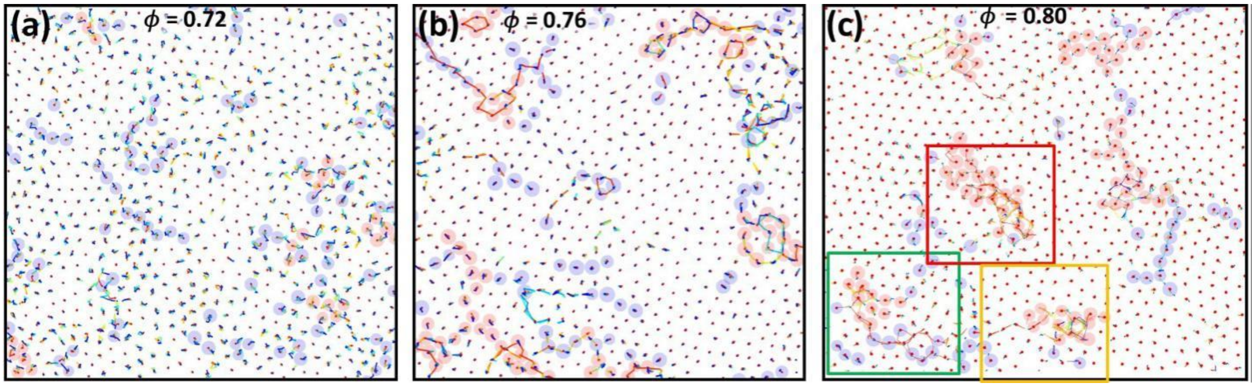


**Figure S18. Experimental Results:** Particle trajectories for duration $T_{traj}$ so that the MSD ≈ $0.2\sigma^2$ for **(a)** $\phi$ = 0.72, **(b)** 0.76, and **(c)** 0.80. The top 15% most mobile particles based on their displacements are shown as circles. Mobile particles classified core-like and string-like are shaded in red and blue respectively.

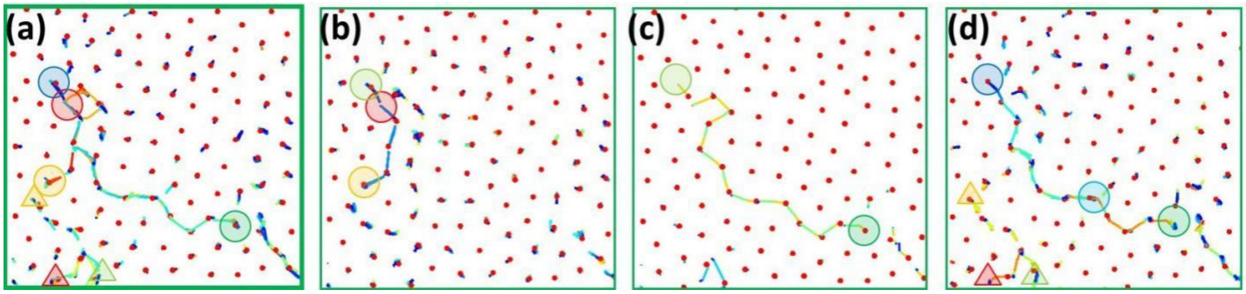


**Figure S19. Experimental Results: (a)** Coarse-grained trajectories from the green box in Figure S18 (c). **(b)-(d)** Consecutive time sequence of coarse-grained trajectories showing details of the dynamics in (a) containing a core-like mobile group. The motions are induced by two quasi-voids denoted by colored circles and triangles.

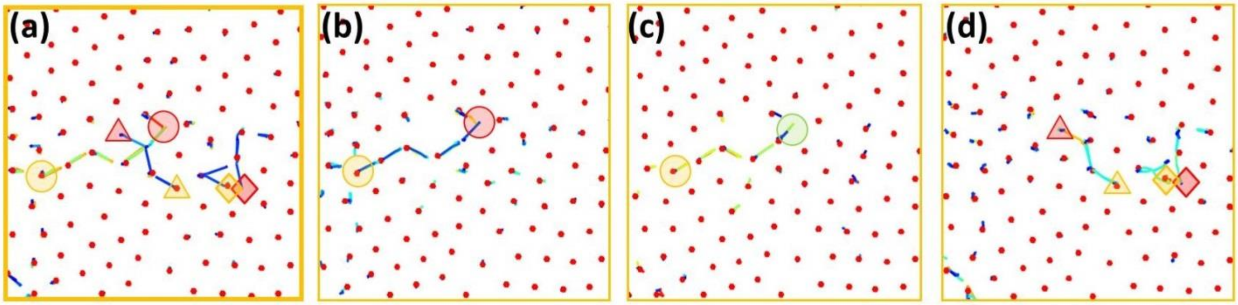


**Figure S20. Experimental Results: (a)** Coarse-grained trajectories from the orange box in Figure S18 (c). **(b)-(d)** Consecutive time sequence of coarse-grained trajectories showing details of the dynamics in (a) containing a core-like mobile group. The motions are induced by three quasi-voids denoted by colored circles, triangles and diamonds.

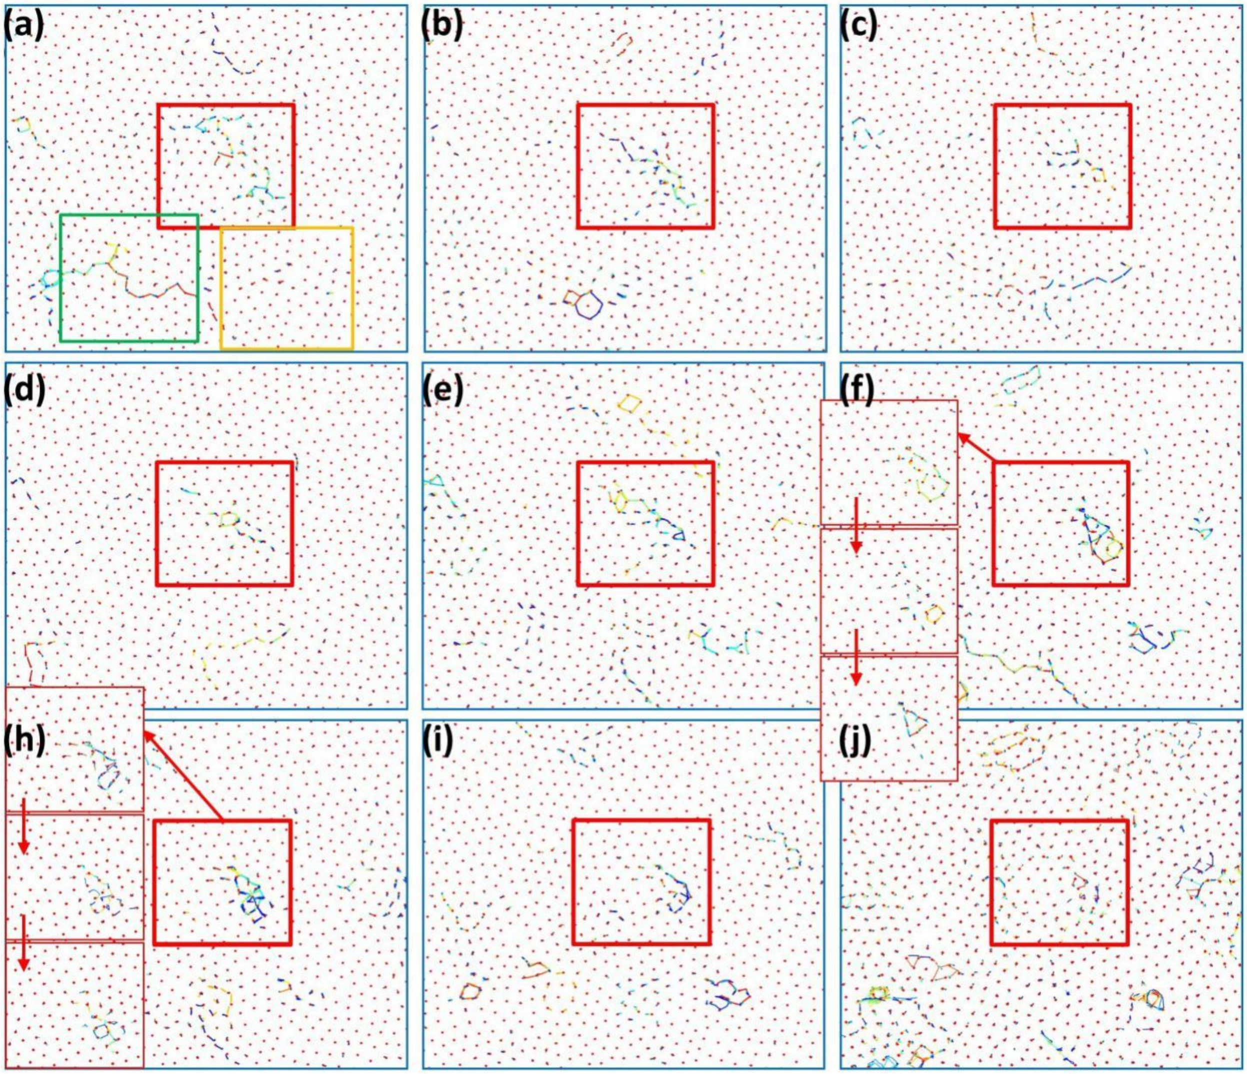


**Figure S21. Experimental Results: (a)** Coarse-grained trajectories from Figure S18 (c). **(b)-(j)** Consecutive time sequence of coarse-grained trajectories showing details of the dynamics in **(a)**. Further details are shown in the insets in (f) and (h).

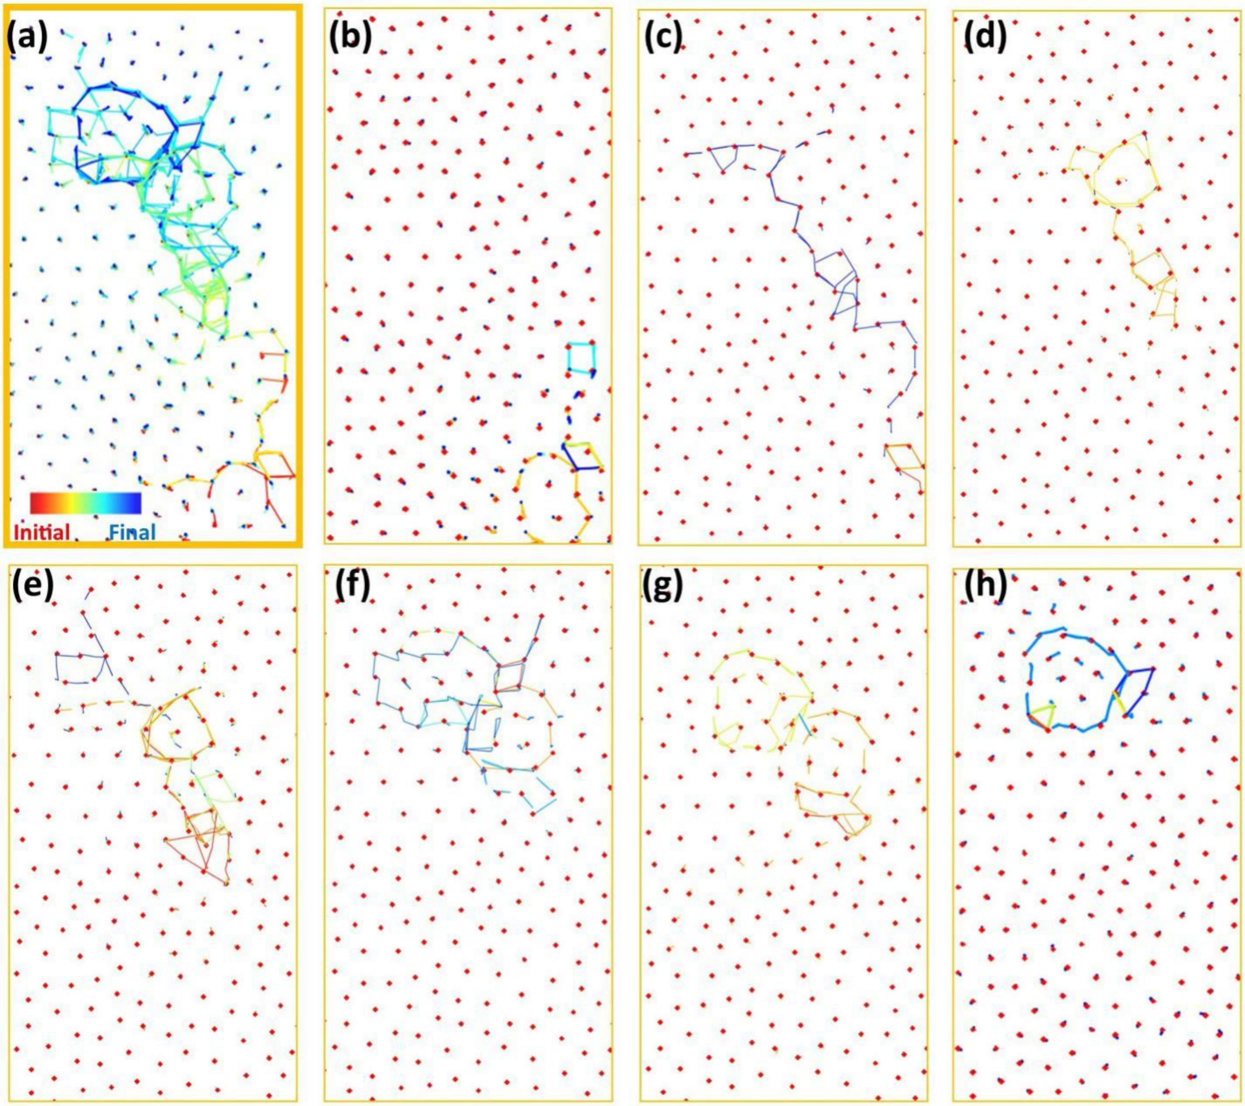


**Figure S22. Simulation Results of packing fraction $\phi_{MD}$ = 0.810: (a)** Coarse-grained trajectories in a region with a core-like mobile cluster. **(b)-(h)** Consecutive time sequence of coarse-grained trajectories showing details of the dynamics in (a).

## 3. Supplementary Results on Glass-Crystal Coexisting Systems

We use unimodal colloidal systems to produce coexisting glassy and crystalline regions for demonstrating the reversible transformation between vacancies and quasi-voids. Once a sample is prepared, it exhibits a fully amorphous state. Then, crystalline regions emerge. After about 8 hours, we observe relatively stable coexisting glassy and crystalline regions. The phase boundaries show no significant evolution during hours of further observations.

We then study particle dynamics in these stabilized glass-crystal coexisting systems as already shown in Figure 2 in the main text. As an additional example, particle trajectories from a similarly prepared sample are shown in Figure S23. In both Figures 2 and S23, we visually identify the glassy and the crystalline regions subjectively. The precise locations of the boundaries may vary slightly if more precise phase identification criteria are used. However, the

existence of both highly ordered and highly disordered regions are evident visually not only from particle arrangements but also from the geometries of the particle trajectories.

From Figure S23(b), trajectories of neighbouring hopping particles join together to form a long string, in a generalized sense, extending from position 1 in the crystalline region to position 2 in the glassy region. The part of the string in the crystalline region takes the geometry of a random walk and is evidently caused by a vacancy. In the glassy region, it is instead generated by the motion of a quasi-void, which is induced by the vacancy as explained in the main text. The quasi-void then moves further to position 3, generating another string-like motion. It is evident that the free volumes of the quasi-void (fragmented blue areas) originate from the vacancy and should be comparable in areas.

We have observed dozens of similar examples of trajectories extending across glassy and crystalline regions in either direction. The alignments of the trajectories are excellent in almost all cases, even across the phase boundary. This is easily explained by introducing quasi-particles referred to as quasi-voids, which can reversibly transform into vacancies. However, such alignments cannot be explained by unorganized generic free volumes supplied by the vacancies. We have observed very long strings at large $\phi$ in the glassy regions generated by the motions of individual quasi-voids. This shows that quasi-voids have long observable lifetimes. This qualifies it as a meaningful quasi-particle for describing glassy dynamics.

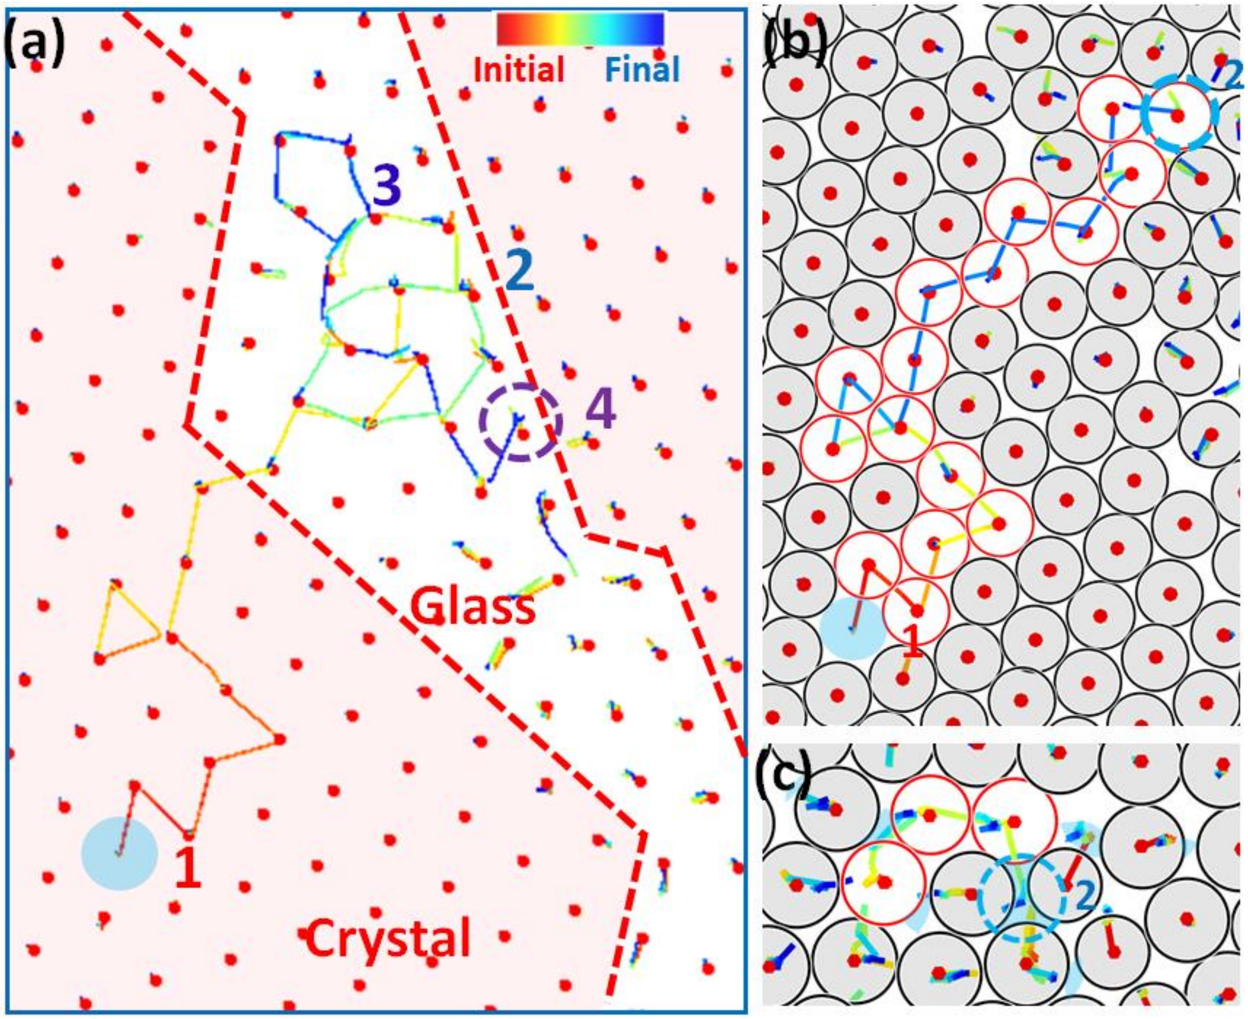


**Figure S23. Experimental Results:** (**a**) Coarse-grained particle trajectories in a coexisting glassy (white) and crystalline (red) system. A vacancy at position 1 induces a quasi-void at position 2 which further moves to position 3. (**b**) and (**c**) Particles and their trajectories showing two consecutive time subintervals of (a). Particles are shown at their initial positions of the subinterval. We observe the conversion of a vacancy (blue circle) into a quasi-void in (b). The resulting quasi-void consisting of fragmented free volumes (blue areas) and a further string-like motion it induces are shown in (c).

**References and Notes:**

31. J. C. Crocker and E. R. Weeks, Particle tracking using IDL (http://www.physics.emory.edu /faculty/weeks//idl/tracking.html).

32. E. P. Bernard, W. Krauth, D. B. Wilson, Event-chain Monte Carlo algorithms for hard-sphere systems, *Phys. Rev. E* **80**, 056704 (2009).

33. M. Isobe, Simple and efficient algorithm for large scale molecular dynamics simulation in hard disk system. *Int. J. Mod. Phys. C* **10**, 1281-1293 (1999).

34. W. G. Hoover, E. Nathan, K. Hanson, Exact hard-disk free volumes. *J. Chem. Phys* **70**, 1837-1844(1979).
